# Supplementary material for: Prediction of Magnetoelectric Multiferroic Janus Monolayers VOXY(X/Y = F, Cl, Br, or I, and X$\not=$Y) with in-plane ferroelectricity and out-of-plane piezoelectricity
Source: arXiv:2208.14203 ancillary file (2022-08-30)
Supplement: Supplementary file 1 [file Supplemental_Material.pdf]

Supplemental Material

# Prediction of Magnetoelectric Multiferroic Janus monolayers VOXY (X/Y = F, Cl, Br, or I, and X≠Y) with in-plane ferroelectricity and out-of-plane piezoelectricity

*Akshay Mahajan* and Somnath Bhowmick#*

Department of Materials Science and Engineering, Indian Institute of Technology Kanpur, Kanpur 208016, India

*E-mail: amahajan@iitk.ac.in

#E-mail: bsomnath@iitk.ac.in

# Figures

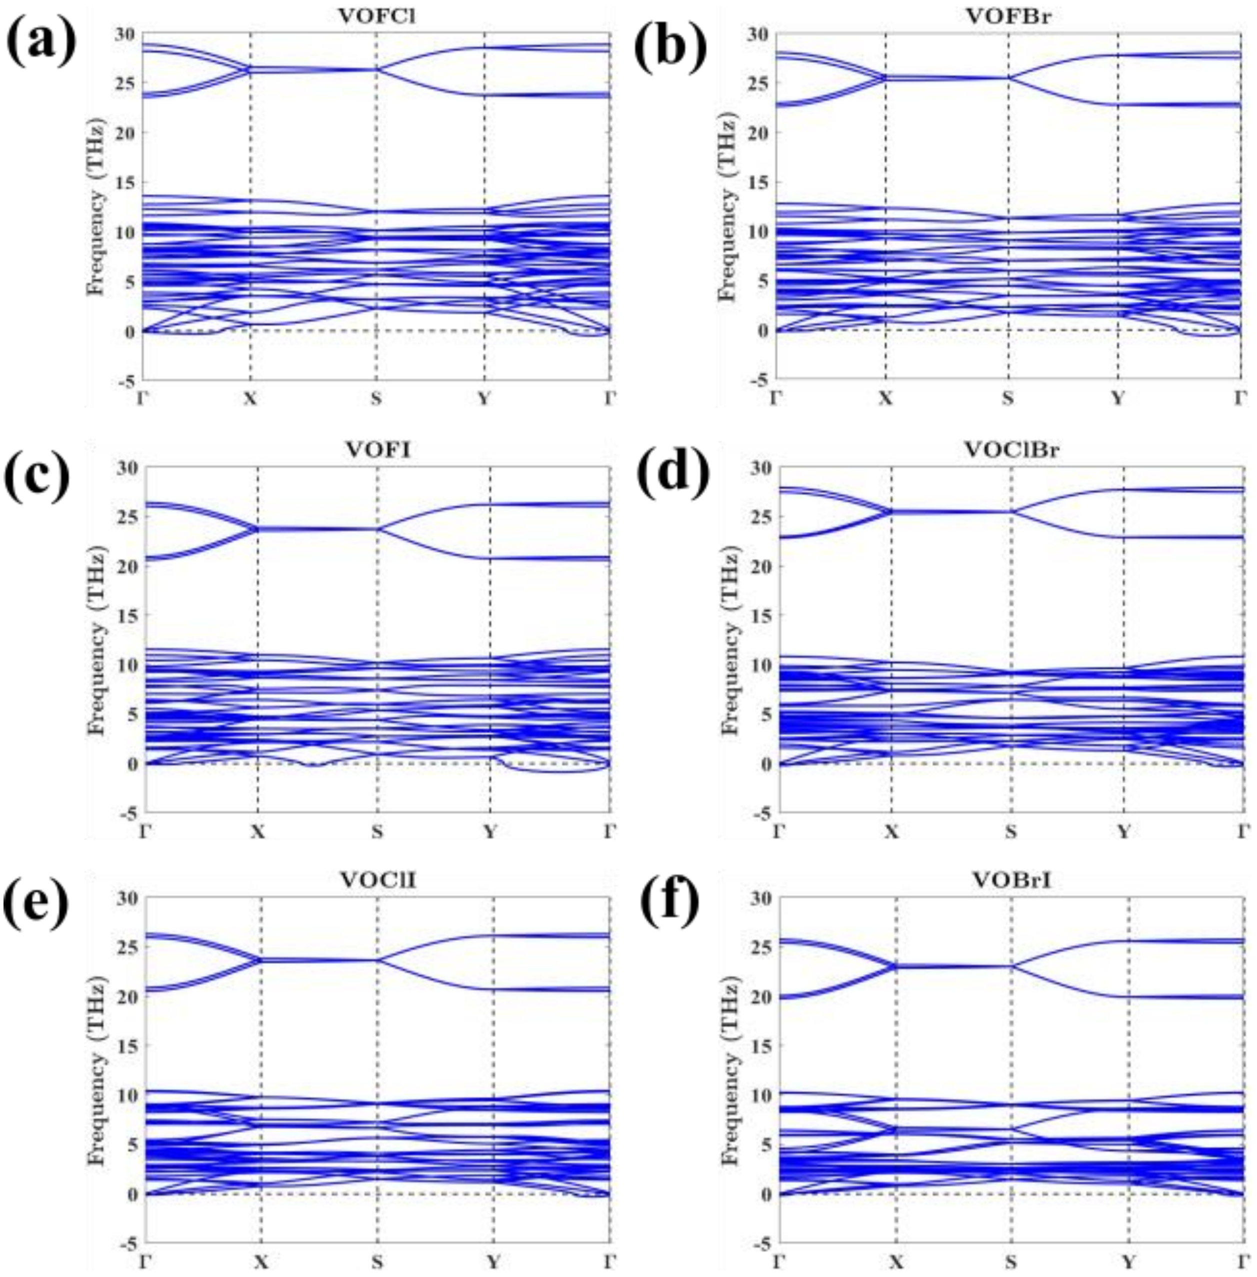


**Figure S1.** Phonon spectra for the Janus VOXY monolayers (a) VOFCl, (b) VOFBr, (c) VOFI, (d) VOClBr, (e) VOClI, and (f) VOBrI.

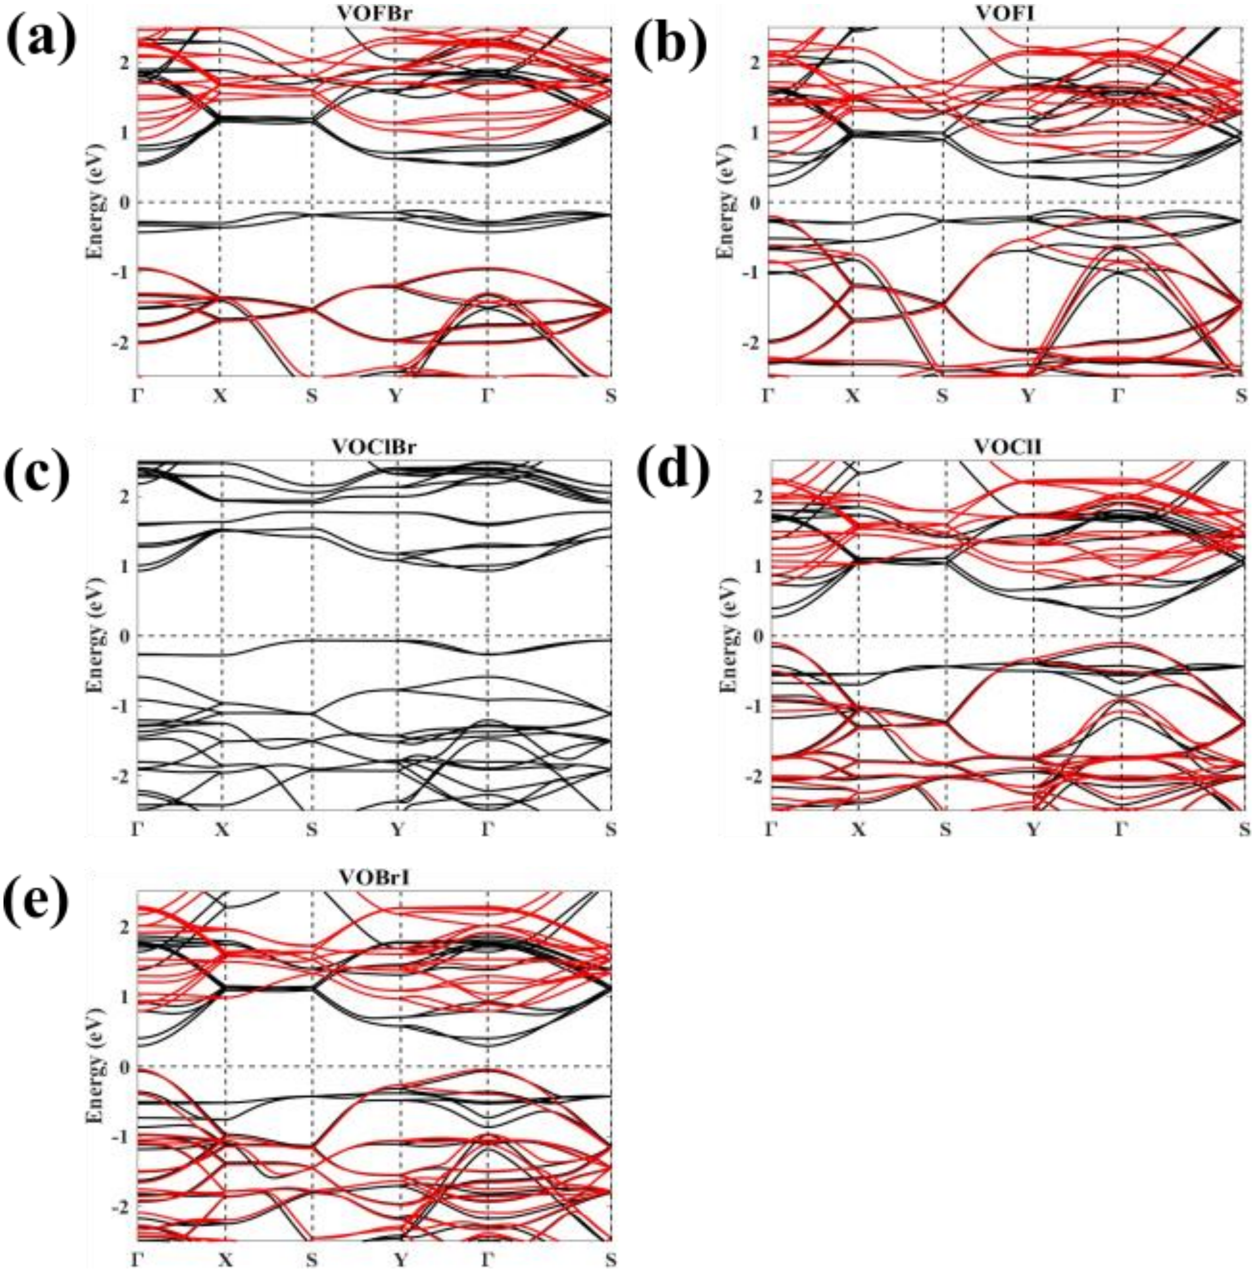


**Figure S2.** Electronic band structure of Janus VOXY monolayers (a) VOFBr, (b) VOFI, (c) VOClBr, (d) VOClI, and (e) VOBrI. Black and red colour bands represent spin-up and spin-down bands, respectively.

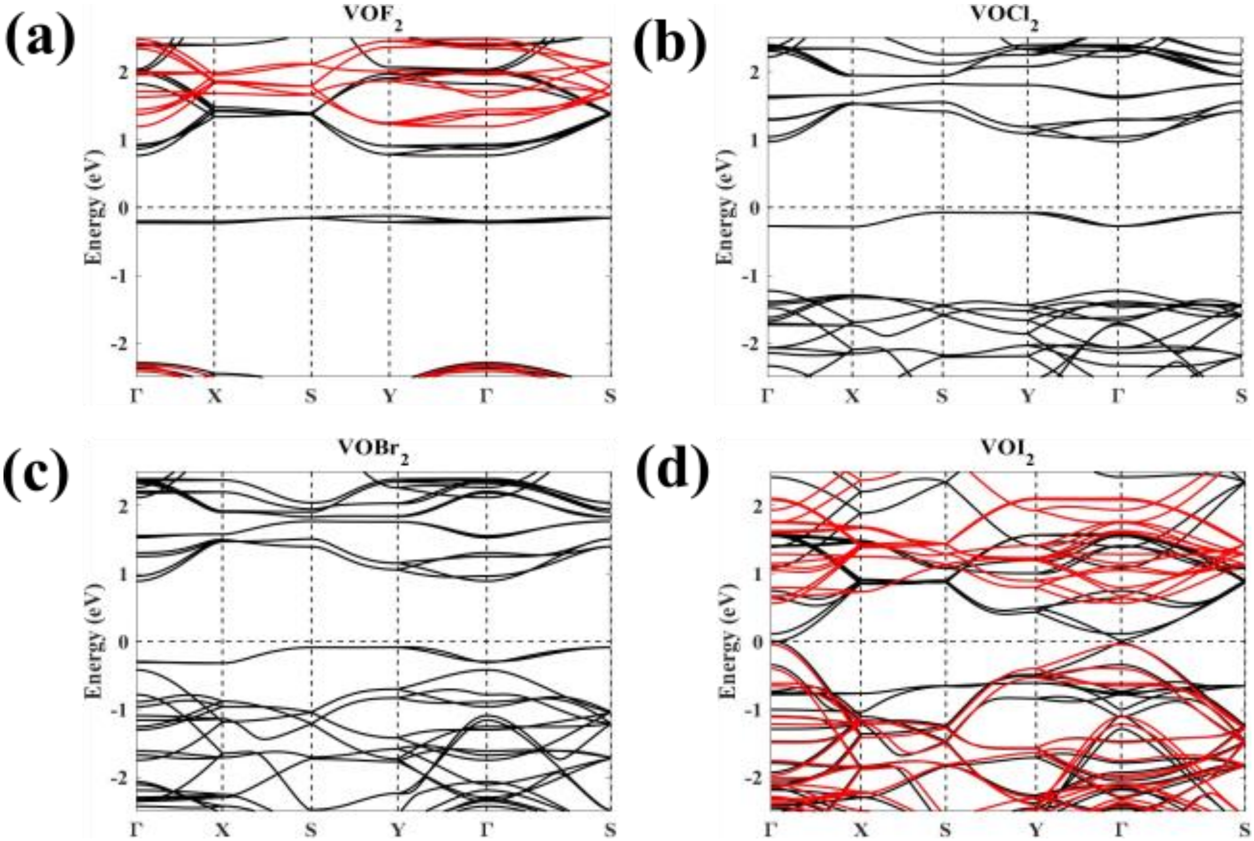


**Figure S3.** Electronic band structure of $VOX_2$ monolayers (a) $VOF_2$, (b) $VOCl_2$, (c) $VOBr_2$, and (d) $VOI_2$. Black and red colour bands represent spin-up and spin-down bands, respectively.

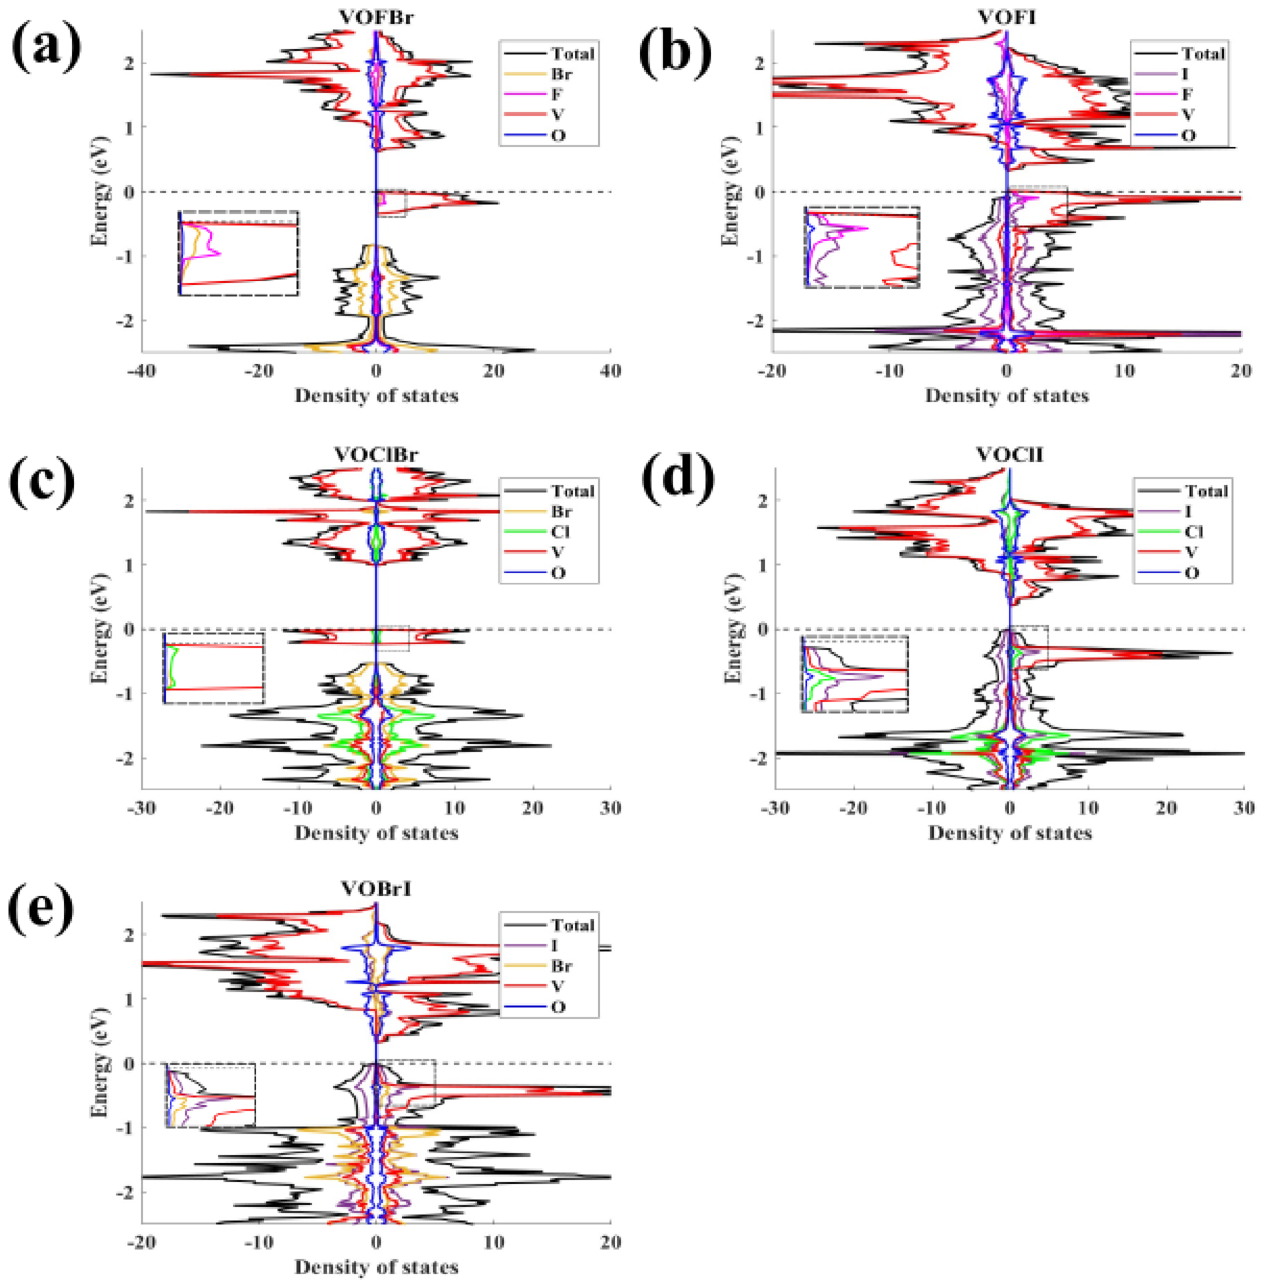


**Figure S4.** Orbital-resolved density of states of Janus VOXY monolayers (a) VOFBr, (b) VOFI, (c) VOClBr, (d) VOClI, and (e) VOBrI. Inset shows the valence states closest to the Fermi level.

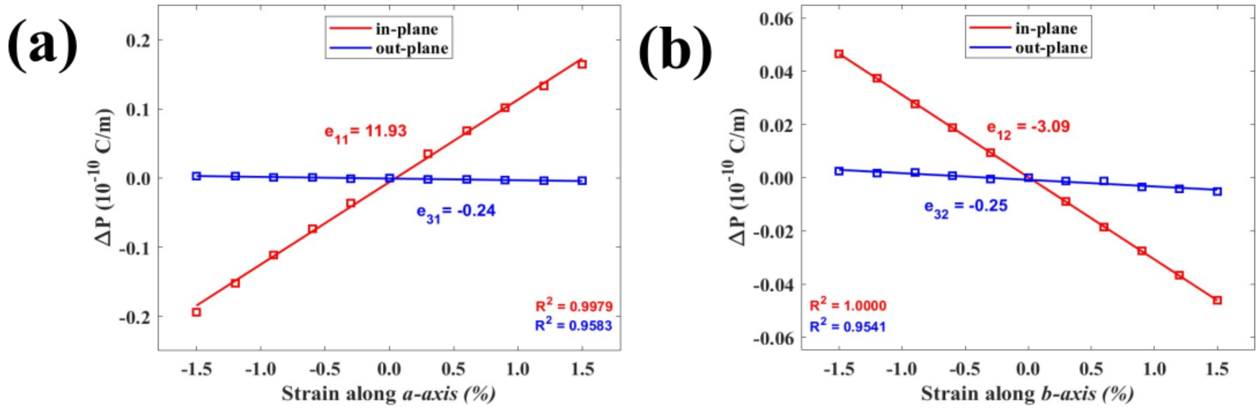


**Figure S5.** Change in the electric polarization for strain (a) along the *a*-axis and (b) along the *b*-axis for the VOFBr monolayer. The slope of the linear fit to the curve provides the monolayer's in-plane (e11 and e12) and out-of-plane (e31 and e32) piezoelectric coefficients. The R-squared values for the linear fit for both in-plane and out-of-plane piezoelectric polarization are provided in the bottom-right and bottom-left corners in (a) and (b), respectively.

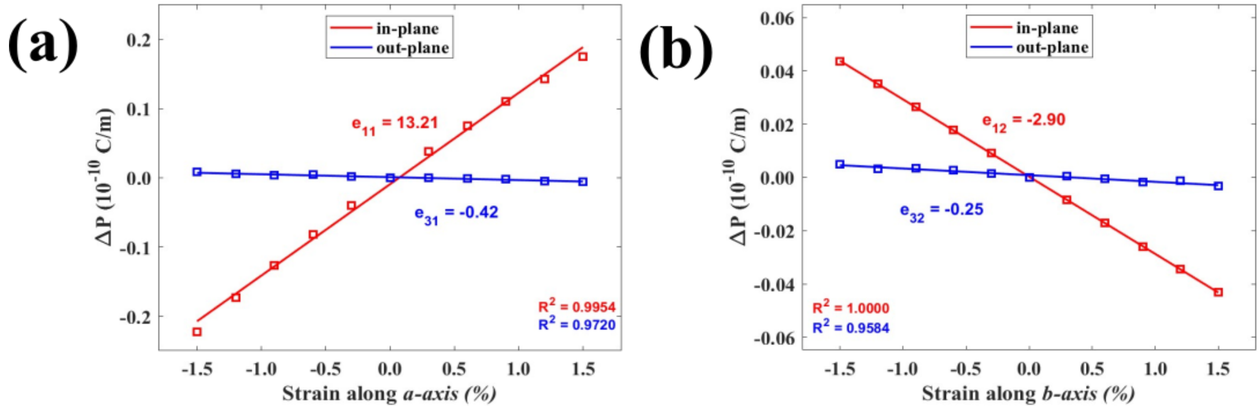


**Figure S6.** Change in the electric polarization for strain (a) along the *a*-axis and (b) along the *b*-axis for the VOFI monolayer. The slope of the linear fit to the curve provides the monolayer's in-plane (e11 and e12) and out-of-plane (e31 and e32) piezoelectric coefficients. The R-squared values for the linear fit for both in-plane and out-of-plane piezoelectric polarization are provided in the bottom-right and bottom-left corners in (a) and (b), respectively.

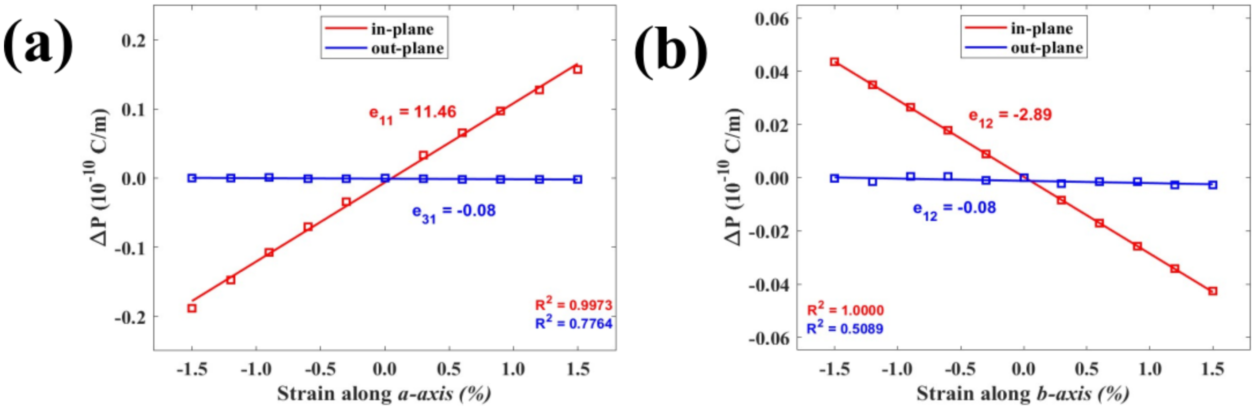


**Figure S7.** Change in the electric polarization for strain (a) along the *a*-axis and (b) along the *b*-axis for the VOClBr monolayer. The slope of the linear fit to the curve provides the monolayer's in-plane (e11 and e12) and out-of-plane (e31 and e32) piezoelectric coefficients. The R-squared values for the linear fit for both in-plane and out-of-plane piezoelectric polarization are provided in the bottom-right and bottom-left corners in (a) and (b), respectively.

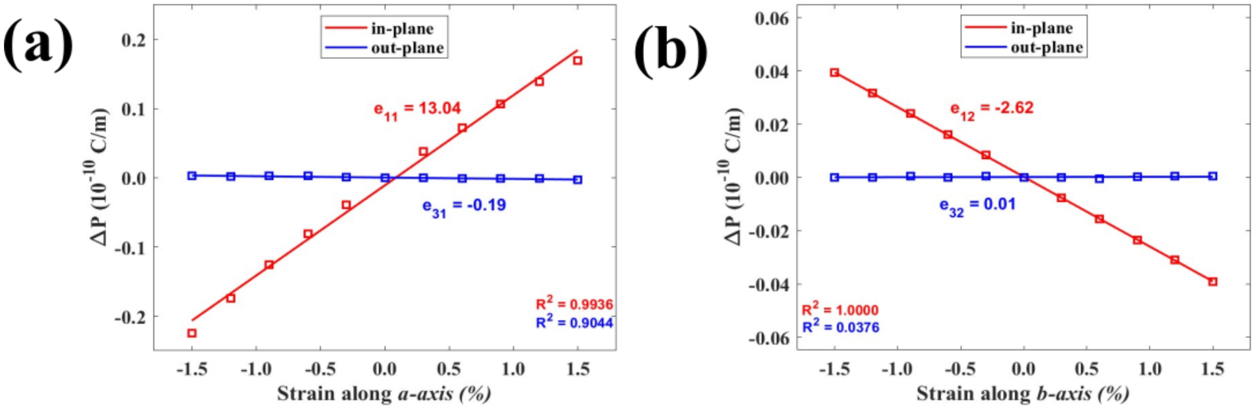


**Figure S8.** Change in the electric polarization for strain (a) along the *a*-axis and (b) along the *b*-axis for the VOClI monolayer. The slope of the linear fit to the curve provides the monolayer's in-plane (e11 and e12) and out-of-plane (e31 and e32) piezoelectric coefficients. The R-squared values for the linear fit for both in-plane and out-of-plane piezoelectric polarization are provided in the bottom-right and bottom-left corners in (a) and (b), respectively.

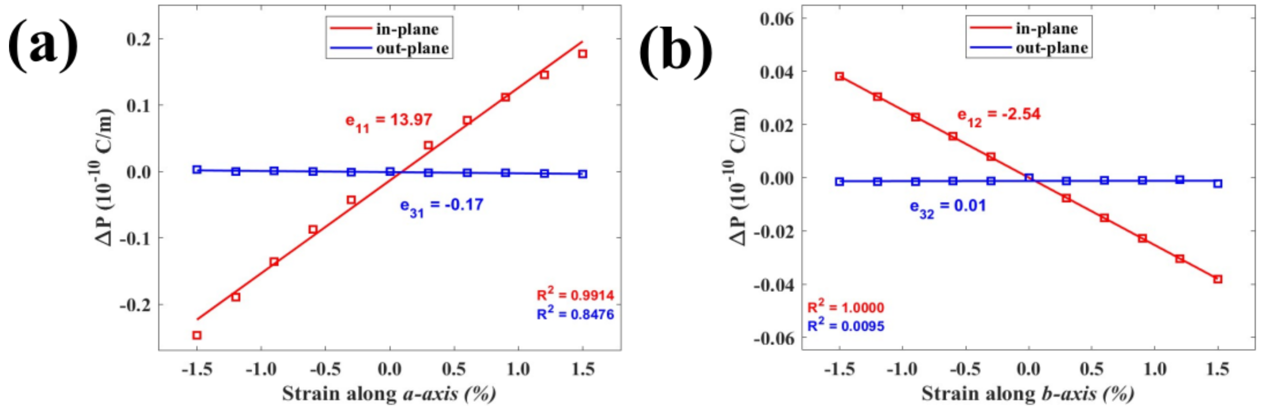


**Figure S9.** Change in the electric polarization for strain (a) along the *a*-axis and (b) along the *b*-axis for the VOBrI monolayer. The slope of the linear fit to the curve provides the monolayer's in-plane (e11 and e12) and out-of-plane (e31 and e32) piezoelectric coefficients. The R-squared values for the linear fit for both in-plane and out-of-plane piezoelectric polarization are provided in the bottom-right and bottom-left corners in (a) and (b), respectively.

# Tables

**Table S1.** Structural parameters of the Janus VOXY and $VOX_2$ monolayers. Here, X and Y are the halogen with higher and lower electronegativity, respectively. P.D. stands for polar displacement of V ion which is given by $\frac{V\text{-}O_2 - V\text{-}O_1}{2}$ .

| | VOFCl | VOFBr | VOFI | VOClBr | VOClI | VOBrI | $VOF_2$ | $VOCl_2$ | $VOBr_2$ | $VOI_2$ |
|---|---|---|---|---|---|---|---|---|---|---|
| ***a*** **(Å)** | 3.801 | 3.795 | 3.806 | 3.806 | 3.814 | 3.814 | 3.818 | 3.810 | 3.805 | 3.811 |
| ***b*** **(Å)** | 3.290 | 3.396 | 3.563 | 3.579 | 3.783 | 3.884 | 3.077 | 3.466 | 3.683 | 4.040 |
| **X-Y (Å)** | 2.907 | 3.033 | 3.176 | 3.507 | 3.633 | 3.779 | 2.507 | 3.375 | 3.648 | 3.962 |
| **V-X (Å)** | 2.028 | 2.043 | 2.067 | 2.446 | 2.464 | 2.622 | 2.001 | 2.435 | 2.606 | 2.838 |
| **V-Y (Å)** | 2.416 | 2.580 | 2.805 | 2.597 | 2.820 | 2.824 | 2.001 | 2.435 | 2.606 | 2.838 |
| **$V\text{-}O_1$ (Å)** | 1.662 | 1.670 | 1.686 | 1.670 | 1.687 | 1.693 | 1.657 | 1.664 | 1.677 | 1.714 |
| **$V\text{-}O_2$ (Å)** | 2.142 | 2.128 | 2.122 | 2.136 | 2.128 | 2.121 | 2.162 | 2.146 | 2.128 | 2.097 |
| **P.D.** | 0.240 | 0.229 | 0.218 | 0.233 | 0.221 | 0.214 | 0.253 | 0.241 | 0.226 | 0.192 |
| **X-V-X** | 108.40 | 112.46 | 119.01 | 94.01 | 100.30 | 95.58 | 100.53 | 90.74 | 89.91 | 90.77 |
| **Y-V-Y** | 85.83 | 82.31 | 78.84 | 87.12 | 84.26 | 86.88 | 100.53 | 90.74 | 89.91 | 90.77 |
| **O-V-O** | 175.19 | 175.51 | 176.87 | 179.76 | 179.17 | 179.36 | 180.00 | 180.00 | 180.00 | 180.00 |

**Table S2.** Lattice parameters *a* and *b* of VOXY monolayers for different magnetic orderings.

| | **VOFCl** | | **VOFBr** | | **VOFI** | |
|---|---|---|---|---|---|---|
| **Magnetic Ordering** | ***a*** **(Å)** | ***b*** **(Å)** | ***a*** **(Å)** | ***b*** **(Å)** | ***a*** **(Å)** | ***b*** **(Å)** |
| AFM1 | 3.804 | 3.276 | 3.797 | 3.392 | 3.807 | 3.563 |
| AFM2 | 3.805 | 3.289 | 3.800 | 3.394 | 3.815 | 3.560 |
| AFM3 | 3.806 | 3.276 | 3.799 | 3.391 | 3.814 | 3.561 |
| FM | 3.801 | 3.290 | 3.795 | 3.396 | 3.806 | 3.563 |

| | **VOClBr** | | **VOClI** | | **VOBrI** | |
|---|---|---|---|---|---|---|
| **Magnetic Ordering** | ***a*** **(Å)** | ***b*** **(Å)** | ***a*** **(Å)** | ***b*** **(Å)** | ***a*** **(Å)** | ***b*** **(Å)** |
| AFM1 | 3.805 | 3.579 | 3.813 | 3.761 | 3.813 | 3.855 |
| AFM2 | 3.805 | 3.620 | 3.821 | 3.780 | 3.821 | 3.881 |
| AFM3 | 3.806 | 3.579 | 3.821 | 3.759 | 3.821 | 3.852 |
| FM | 3.802 | 3.622 | 3.814 | 3.783 | 3.814 | 3.884 |

**Table S3.** Lattice parameters *a* and *b* of $VOX_2$ monolayers for different magnetic orderings.

| | $VOF_2$ | | $VOCl_2$ | | $VOBr_2$ | | $VOI_2$ | |
|---|---|---|---|---|---|---|---|---|
| **Magnetic Ordering** | ***a* (Å)** | ***b* (Å)** | ***a* (Å)** | ***b* (Å)** | ***a* (Å)** | ***b* (Å)** | ***a* (Å)** | ***b* (Å)** |
| AFM1 | 3.822 | 3.064 | 3.810 | 3.466 | 3.803 | 3.682 | 3.823 | 4.006 |
| AFM2 | 3.820 | 3.076 | 3.807 | 3.516 | 3.804 | 3.724 | 3.840 | 4.031 |
| AFM3 | 3.821 | 3.064 | 3.810 | 3.466 | 3.805 | 3.682 | 3.839 | 4.001 |
| FM | 3.818 | 3.077 | 3.805 | 3.518 | 3.801 | 3.725 | 3.811 | 4.040 |

# Crystal Structures

**POSCAR-VOFCl (FM)**

```
VOFCl-FM
   1.00000000000000
     7.6019782042697379    0.0000000000000000    0.0000000000000000
     0.0000000000000000    6.5802591908210024    0.0000000000000000
     0.0000000000000000    0.0000000000000000   23.7377605438000003
   Cl   F    V    O
     4    4    4    4
Direct
  0.9994412860975098  0.2500000000000000  0.4316737595795623
  0.9994412860975098  0.7500000340000028  0.4316737595795623
  0.4994412860975094  0.2500000000000000  0.4316737595795623
  0.4994412860975094  0.7500000340000028  0.4316737595795623
  0.9982045109399083  0.2500000000000000  0.5541571535458948
  0.9982045109399083  0.7500000340000028  0.5541571535458948
  0.4982045109399081  0.2500000000000000  0.5541571535458948
  0.4982045109399081  0.7500000340000028  0.5541571535458948
  0.0330338593664067  0.0000000000000000  0.5054298398022907
  0.0330338593664067  0.5000000000000000  0.5054298398022907
  0.5330338593664067  0.0000000000000000  0.5054298398022907
  0.5330338593664067  0.5000000000000000  0.5054298398022907
  0.2514650433090843 -0.0000000000000000  0.5087392470722593
  0.2514650433090843  0.5000000000000000  0.5087392470722593
  0.7514650433090843 -0.0000000000000000  0.5087392470722593
  0.7514650433090843  0.5000000000000000  0.5087392470722593
```

**POSCAR-VOFBr (FM)**

```
VOFBr-FM
   1.00000000000000
     7.5896642324959913    0.0000000000000000    0.0000000000000000
     0.0000000000000000    6.7917413169176628    0.0000000000000000
     0.0000000000000000    0.0000000000000000   23.7377605438000003
   Br   F    V    O
     4     4     4     4
Direct
  0.9988620345722780  0.2500000000000000  0.4267077085006589
  0.9988620345722780  0.7500000340000028  0.4267077085006589
  0.4988620345722778  0.2500000000000000  0.4267077085006589
  0.4988620345722778  0.7500000340000028  0.4267077085006589
  0.9979571845166337  0.2500000000000000  0.5544647967780328
  0.9979571845166337  0.7500000340000028  0.5544647967780328
  0.4979571845166340  0.2500000000000000  0.5544647967780328
  0.4979571845166340  0.7500000340000028  0.5544647967780328
  0.0317235284307762  0.0000000000000000  0.5078695405413832
  0.0317235284307762  0.5000000000000000  0.5078695405413832
  0.5317235284307763  0.0000000000000000  0.5078695405413832
  0.5317235284307763  0.5000000000000000  0.5078695405413832
  0.2515103393650964  0.0000000000000000  0.5109579541799110
  0.2515103393650964  0.5000000000000000  0.5109579541799110
  0.7515103393650964  0.0000000000000000  0.5109579541799110
  0.7515103393650964  0.5000000000000000  0.5109579541799110
```

**POSCAR-VOFI (FM)**

```
VOFI-FM
   1.00000000000000
     7.6121142295209934    0.0000000000000000    0.0000000000000000
     0.0000000000000000    7.1261931922029316    0.0000000000000000
     0.0000000000000000    0.0000000000000000   23.7377605438000003
   I    F    V    O
     4     4     4     4
Direct
  0.9982888369036658  0.2500000000000000  0.4206254004665619
  0.9982888369036658  0.7500000340000028  0.4206254004665619
  0.4982888369036657  0.2500000000000000  0.4206254004665619
  0.4982888369036657  0.7500000340000028  0.4206254004665619
  0.9970793934568259  0.2500000000000000  0.5544124256094002
  0.9970793934568259  0.7500000340000028  0.5544124256094002
  0.4970793934568187  0.2500000000000000  0.5544124256094002
  0.4970793934568187  0.7500000340000028  0.5544124256094002
  0.0288170608217444  0.0000000000000000  0.5113993390388938
  0.0288170608217444  0.5000000000000000  0.5113993390388938
  0.5288170608217445  0.0000000000000000  0.5113993390388938
  0.5288170608217445  0.5000000000000000  0.5113993390388938
  0.2501410444620463  0.0000000000000000  0.5135628348851446
  0.2501410444620463  0.5000000000000000  0.5135628348851446
  0.7501410444620462  0.0000000000000000  0.5135628348851446
  0.7501410444620462  0.5000000000000000  0.5135628348851446
```

**POSCAR-VOClBr (AFM3)**

```
VOClBr-AFM3
   1.00000000000000
     7.6123100132549801    0.0000000000000000    0.0000000000000000
     0.0000000000000000    7.1576685554691934    0.0000000000000000
     0.0000000000000000    0.0000000000000000   26.2990818023999999
   Br   Cl   V    O
     4     4     4     4
Direct
  0.9969811428886535  0.2500000000000000  0.4313098194768220
  0.9969811428886535  0.7499999839999987  0.4313098194768220
  0.4969811428886537  0.2500000000000000  0.4313098194768220
  0.4969811428886537  0.7499999839999987  0.4313098194768220
  0.9974769439037899  0.2500000000000000  0.5646677238333898
  0.9974769439037899  0.7499999839999987  0.5646677238333898
  0.4974769439037902  0.2500000000000000  0.5646677238333898
  0.4974769439037902  0.7499999839999987  0.5646677238333898
  0.0333417692504149 -0.0000000000000000  0.5020848677164440
  0.0333417692504149  0.5000000000000000  0.5020848677164440
  0.5333417692504078 -0.0000000000000000  0.5020848677164440
  0.5333417692504078  0.5000000000000000  0.5020848677164440
  0.2527598150459226 -0.0000000000000000  0.5019375889733442
  0.2527598150459226  0.5000000000000000  0.5019375889733442
  0.7527597990459212 -0.0000000000000000  0.5019375889733442
  0.7527597990459212  0.5000000000000000  0.5019375889733442
```

**POSCAR-VOClI (FM)**

```
VOClI-FM
   1.00000000000000
     7.6285037032480769    0.0000000000000000    0.0000000000000000
     0.0000000000000000    7.5659236034383834    0.0000000000000000
     0.0000000000000000    0.0000000000000000   23.7377605438000003
   I    Cl   V    O
     4     4     4     4
Direct
  0.9964935803293642  0.2500000000000000  0.4181653186730969
  0.9964935803293642  0.7500000340000028  0.4181653186730969
  0.4964935803293642  0.2500000000000000  0.4181653186730969
  0.4964935803293642  0.7500000340000028  0.4181653186730969
  0.9966470956942857  0.2500000000000000  0.5712255037576313
  0.9966470956942857  0.7500000340000028  0.5712255037576313
  0.4966470956942857  0.2500000000000000  0.5712255037576313
  0.4966470956942857  0.7500000340000028  0.5712255037576313
  0.0300436485025912  0.0000000000000000  0.5055910787723974
  0.0300436485025912  0.5000000000000000  0.5055910787723974
  0.5300436485025912  0.0000000000000000  0.5055910787723974
  0.5300436485025912  0.5000000000000000  0.5055910787723974
  0.2511420111180342  0.0000000000000000  0.5050180987968815
  0.2511420111180342  0.5000000000000000  0.5050180987968815
  0.7511420111180342  0.0000000000000000  0.5050180987968815
  0.7511420111180342  0.5000000000000000  0.5050180987968815
```

## **POSCAR-VOBrI (FM)**

```
VOBrI-FM
   1.00000000000000
     7.6280951776303283    0.0000000000000000    0.0000000000000000
     0.0000000000000000    7.7689855607764695    0.0000000000000000
     0.0000000000000000    0.0000000000000000   23.7377605438000003
   I    Br   V    O
     4     4     4     4
Direct
  0.9969132872175951  0.2500000000000000  0.4174286396982066
  0.9969132872175951  0.7500000340000028  0.4174286396982066
  0.4969132872175952  0.2500000000000000  0.4174286396982066
  0.4969132872175952  0.7500000340000028  0.4174286396982066
  0.9964828751791063  0.2500000000000000  0.5766441656298374
  0.9964828751791063  0.7500000340000028  0.5766441656298374
  0.4964828751791064  0.2500000000000000  0.5766441656298374
  0.4964828751791064  0.7500000340000028  0.5766441656298374
  0.0294753586128165  0.0000000000000000  0.5031836158398901
  0.0294753586128165  0.5000000000000000  0.5031836158398901
  0.5294753586128164 -0.0000000000000000  0.5031836158398901
  0.5294753586128164  0.5000000000000000  0.5031836158398901
  0.2514548146347646 -0.0000000000000000  0.5027435788320594
  0.2514548146347646  0.5000000000000000  0.5027435788320594
  0.7514548146347646 -0.0000000000000000  0.5027435788320594
  0.7514548146347646  0.5000000000000000  0.5027435788320594
```

## **POSCAR-$VOF_2$ (FM)**

```
VOF2-FM
   1.00000000000000
     7.6366697171333930    0.0000000000000000    0.0000000000000000
     0.0000000000000000    6.1535078475872940    0.0000000000000000
     0.0000000000000000    0.0000000000000000   23.7377605438000003
   F    V    O
     8     4     4
Direct
 -0.0001470302160661  0.2500000000000000  0.4472031332273798
 -0.0001470302160661  0.7500000340000028  0.4472031332273798
  0.4998529697839341  0.2500000000000000  0.4472031332273798
  0.4998529697839341  0.7500000340000028  0.4472031332273798
 -0.0001470302160661  0.2500000000000000  0.5527968667726204
 -0.0001470302160661  0.7500000340000028  0.5527968667726204
  0.4998529697839341  0.2500000000000000  0.5527968667726204
  0.4998529697839341  0.7500000340000028  0.5527968667726204
  0.0331378935636455 -0.0000000000000000  0.5000000000000000
  0.0331378935636455  0.5000000000000000  0.5000000000000000
  0.5331378935636455 -0.0000000000000000  0.5000000000000000
  0.5331378935636455  0.5000000000000000  0.5000000000000000
  0.2501369777920766 -0.0000000000000000  0.5000000000000000
  0.2501369777920766  0.5000000000000000  0.5000000000000000
  0.7501369777920767 -0.0000000000000000  0.5000000000000000
  0.7501369777920767  0.5000000000000000  0.5000000000000000
```

**POSCAR-$VOCl_2$ (AFM3)**

```
VOCl2-AFM3
   1.00000000000000
     7.6200175939177619    0.0000000000000000    0.0000000000000000
     0.0000000000000000    6.9314913139799064    0.0000000000000000
     0.0000000000000000    0.0000000000000000   23.7377605438000003
   Cl   V    O
     8     4     4
Direct
  0.9976671567572419  0.2500000000000000  0.4289135342457537
  0.9976671567572419  0.7500000850000035  0.4289135342457537
  0.4976671567572420  0.2500000000000000  0.4289135342457537
  0.4976671567572420  0.7500000850000035  0.4289135342457537
  0.9976671567572419  0.2500000000000000  0.5710864657542462
  0.9976671567572419  0.7500000850000035  0.5710864657542462
  0.4976671567572420  0.2500000000000000  0.5710864657542462
  0.4976671567572420  0.7500000850000035  0.5710864657542462
  0.0345350260108641  0.0000000000000000  0.5000000000000000
  0.0345350260108641  0.5000000000000000  0.5000000000000000
  0.5345350260108642  0.0000000000000000  0.5000000000000000
  0.5345350260108642  0.5000000000000000  0.5000000000000000
  0.2528517769641567  0.0000000000000000  0.5000000000000000
  0.2528517769641567  0.5000000000000000  0.5000000000000000
  0.7528517439641575  0.0000000000000000  0.5000000000000000
  0.7528517439641575  0.5000000000000000  0.5000000000000000
```

**POSCAR-$VOBr_2$ (AFM3)**

```
VOBr2-AFM3
   1.00000000000000
     7.6102068731931887    0.0000000000000000    0.0000000000000000
     0.0000000000000000    7.3650879397211622    0.0000000000000000
     0.0000000000000000    0.0000000000000000   23.7377605438000003
   Br   V    O
     8     4     4
Direct
  0.9972566191723108  0.2500000000000000  0.4231530803269784
  0.9972566191723108  0.7500000850000035  0.4231530803269784
  0.4972566191723107  0.2500000000000000  0.4231530803269784
  0.4972566191723107  0.7500000850000035  0.4231530803269784
  0.9972566191723108  0.2500000000000000  0.5768469196730286
  0.9972566191723108  0.7500000850000035  0.5768469196730286
  0.4972566191723107  0.2500000000000000  0.5768469196730286
  0.4972566191723107  0.7500000850000035  0.5768469196730286
  0.0327292555763634  0.0000000000000000  0.5000000000000000
  0.0327292555763634  0.5000000000000000  0.5000000000000000
  0.5327292555763633  0.0000000000000000  0.5000000000000000
  0.5327292555763633  0.5000000000000000  0.5000000000000000
  0.2530602783439329  0.0000000000000000  0.5000000000000000
  0.2530602783439329  0.5000000000000000  0.5000000000000000
  0.7530602453439336 -0.0000000000000000  0.5000000000000000
  0.7530602453439336  0.5000000000000000  0.5000000000000000
```

| POSCAR-$VOI_2$ (FM) |
|---|
| VOI2-FM<br>1.00000000000000<br>7.6217600878564520 0.0000000000000000 0.0000000000000000<br>0.0000000000000000 8.0797954412011190 0.0000000000000000<br>0.0000000000000000 0.0000000000000000 23.7377605438000003<br>I V O<br>8 4 4<br>Direct<br>0.9980205248719054 0.2500000000000000 0.4165542107440776<br>0.9980205248719054 0.7500000340000028 0.4165542107440776<br>0.4980205248719056 0.2500000000000000 0.4165542107440776<br>0.4980205248719056 0.7500000340000028 0.4165542107440776<br>0.9980205248719054 0.2500000000000000 0.5834457892559223<br>0.9980205248719054 0.7500000340000028 0.5834457892559223<br>0.4980205248719056 0.2500000000000000 0.5834457892559223<br>0.4980205248719056 0.7500000340000028 0.5834457892559223<br>0.0266826314936607 -0.0000000000000000 0.5000000000000000<br>0.0266826314936607 0.5000000000000000 0.5000000000000000<br>0.5266826314936607 -0.0000000000000000 0.5000000000000000<br>0.5266826314936607 0.5000000000000000 0.5000000000000000<br>0.2516026544067893 -0.0000000000000000 0.5000000000000000<br>0.2516026544067893 0.5000000000000000 0.5000000000000000<br>0.7516026544067893 -0.0000000000000000 0.5000000000000000<br>0.7516026544067893 0.5000000000000000 0.5000000000000000 |

# Additional Note on Electric Polarization Calculation

Within the modern theory of polarization [1], ferroelectric polarization is calculated by taking the difference between the electric dipole moment of the low symmetry ferroelectric (FE) phase and the high-symmetric paraelectric (PE) phase. In VASP, using the LCALCPOL tag, ionic and electronic dipole moments were calculated in all three cartesian directions, and the in-plane ferroelectric polarization was calculated by taking the dipole moment value for the high-symmetric PE phase as the reference point. It was observed that the PE phase of the monolayers with FM spin-ordering shows metallic nature within the approximations used in the present DFT calculations. The berry phase calculation for getting electric dipole moment is possible only for an insulating material system within LCALCPOL's formalism. To resolve this issue, we used the DFT+U approach [2] using different $U_{eff}$ values that has a Mott nature and thus lifts the bands in the PE phase for FM magnetic ordering, opening a band gap and thus making it possible to calculate the dipole moments. The ionic dipole moment remains unaffected by using different $U_{eff}$ values, while the electronic dipole moment changes. Interestingly, for PE

phase of FM monolayers, the electronic dipole moment remains constant to zero along the polar axis of the ferroelectric polarization (*a*-axis) for different $U_{eff}$ values. Thus, the dipole moment values for the PE phase of FM-ordered monolayers calculated using the DFT+U approach can be used as a reference for in-plane ferroelectric polarization in this work, where DFT+U is not incorporated for the FE phase of the monolayers.

*References -:*


[1] N. A. Spaldin, *A Beginner's Guide to the Modern Theory of Polarization*, Journal of Solid State Chemistry **195**, 2 (2012).

[2] S. L. Dudarev, G. A. Botton, S. Y. Savrasov, C. J. Humphreys, and A. P. Sutton, *Electron-Energy-Loss Spectra and the Structural Stability of Nickel Oxide: An LSDA+U Study*, Phys. Rev. B **57**, 1505 (1998).
